# Supplementary material for: Mitigating the Impact of Outlier Channels for Language Model Quantization with Activation Regularization
Source: arXiv:2404.03605 source file (2024-08-26)
Supplement: Supplementary file 1 [file appendix.tex]

\section{Appendix}

\begin{table*}[t!]\centering
\footnotesize
% \ra{1.3}
\begin{tabular}{@{}rrrcrrrr@{}}\toprule
& \multicolumn{2}{c}{Native Activations} & \phantom{abc}& \multicolumn{4}{c}{4b Activations} \\
\cmidrule{2-3} \cmidrule{5-8}
Weight Precision & 16 &  4 && 4 & 4 & 3 & 3  \\ 
Weight Quantizer &None &GPTQ&&GPTQ&RTN&GPTQ&RTN \\
\midrule
\textbf{C4}\\
\textit{Baseline} & 29.23 & 30.36 && 4288 & 3864 & 4820.5 & 3923.96 \\ 
\textit{QAT} & 30.25 & 31.30 && 31.30 & 32.55 & 36.47 & 44.73 \\ 
\textit{QAT+Kurtosis Reg.} & 29.95 & 30.83 && 30.83 & 31.73 & 35.47 & 45.04 \\ 
 \midrule
 \textbf{PTB}\\
\textit{Baseline}& 32.61 & 34.12 && 2974 & 2896 & 3767 & 2950 \\
\textit{QAT} & 33.56 & 34.83 && 34.83 & 34.24 & 47.51 & 51.22 \\
\textit{QAT+ Kurtosis Reg.}& 33.14 & 34.23 && 34.23 & 34.55 & 40.74 & 52.63 \\
\bottomrule
\end{tabular}
\vspace{-2mm}
\caption{Perplexity results of 300M models on C4 (top) and PTB (bottom). Native activation bits are 16 bits for \textit{Baseline}, \textit{Activation Clamping}, and \textit{Kurtosis Reglarization}, and 4 bits for \textit{QAT } and \textit{ QAT + Kurtosis Regularization}. }
\label{tab:300M}
\vspace{-2mm}
\end{table*}
